# Supplementary material for: Movie101v2: Improved Movie Narration Benchmark
Source: arXiv:2404.13370 source file (2024-10-18)
Supplement: Supplementary file 2 [file supp-qualitative-zh.tex]

\begin{figure*}[t]
    \begin{center}
        \includegraphics[width=\linewidth]{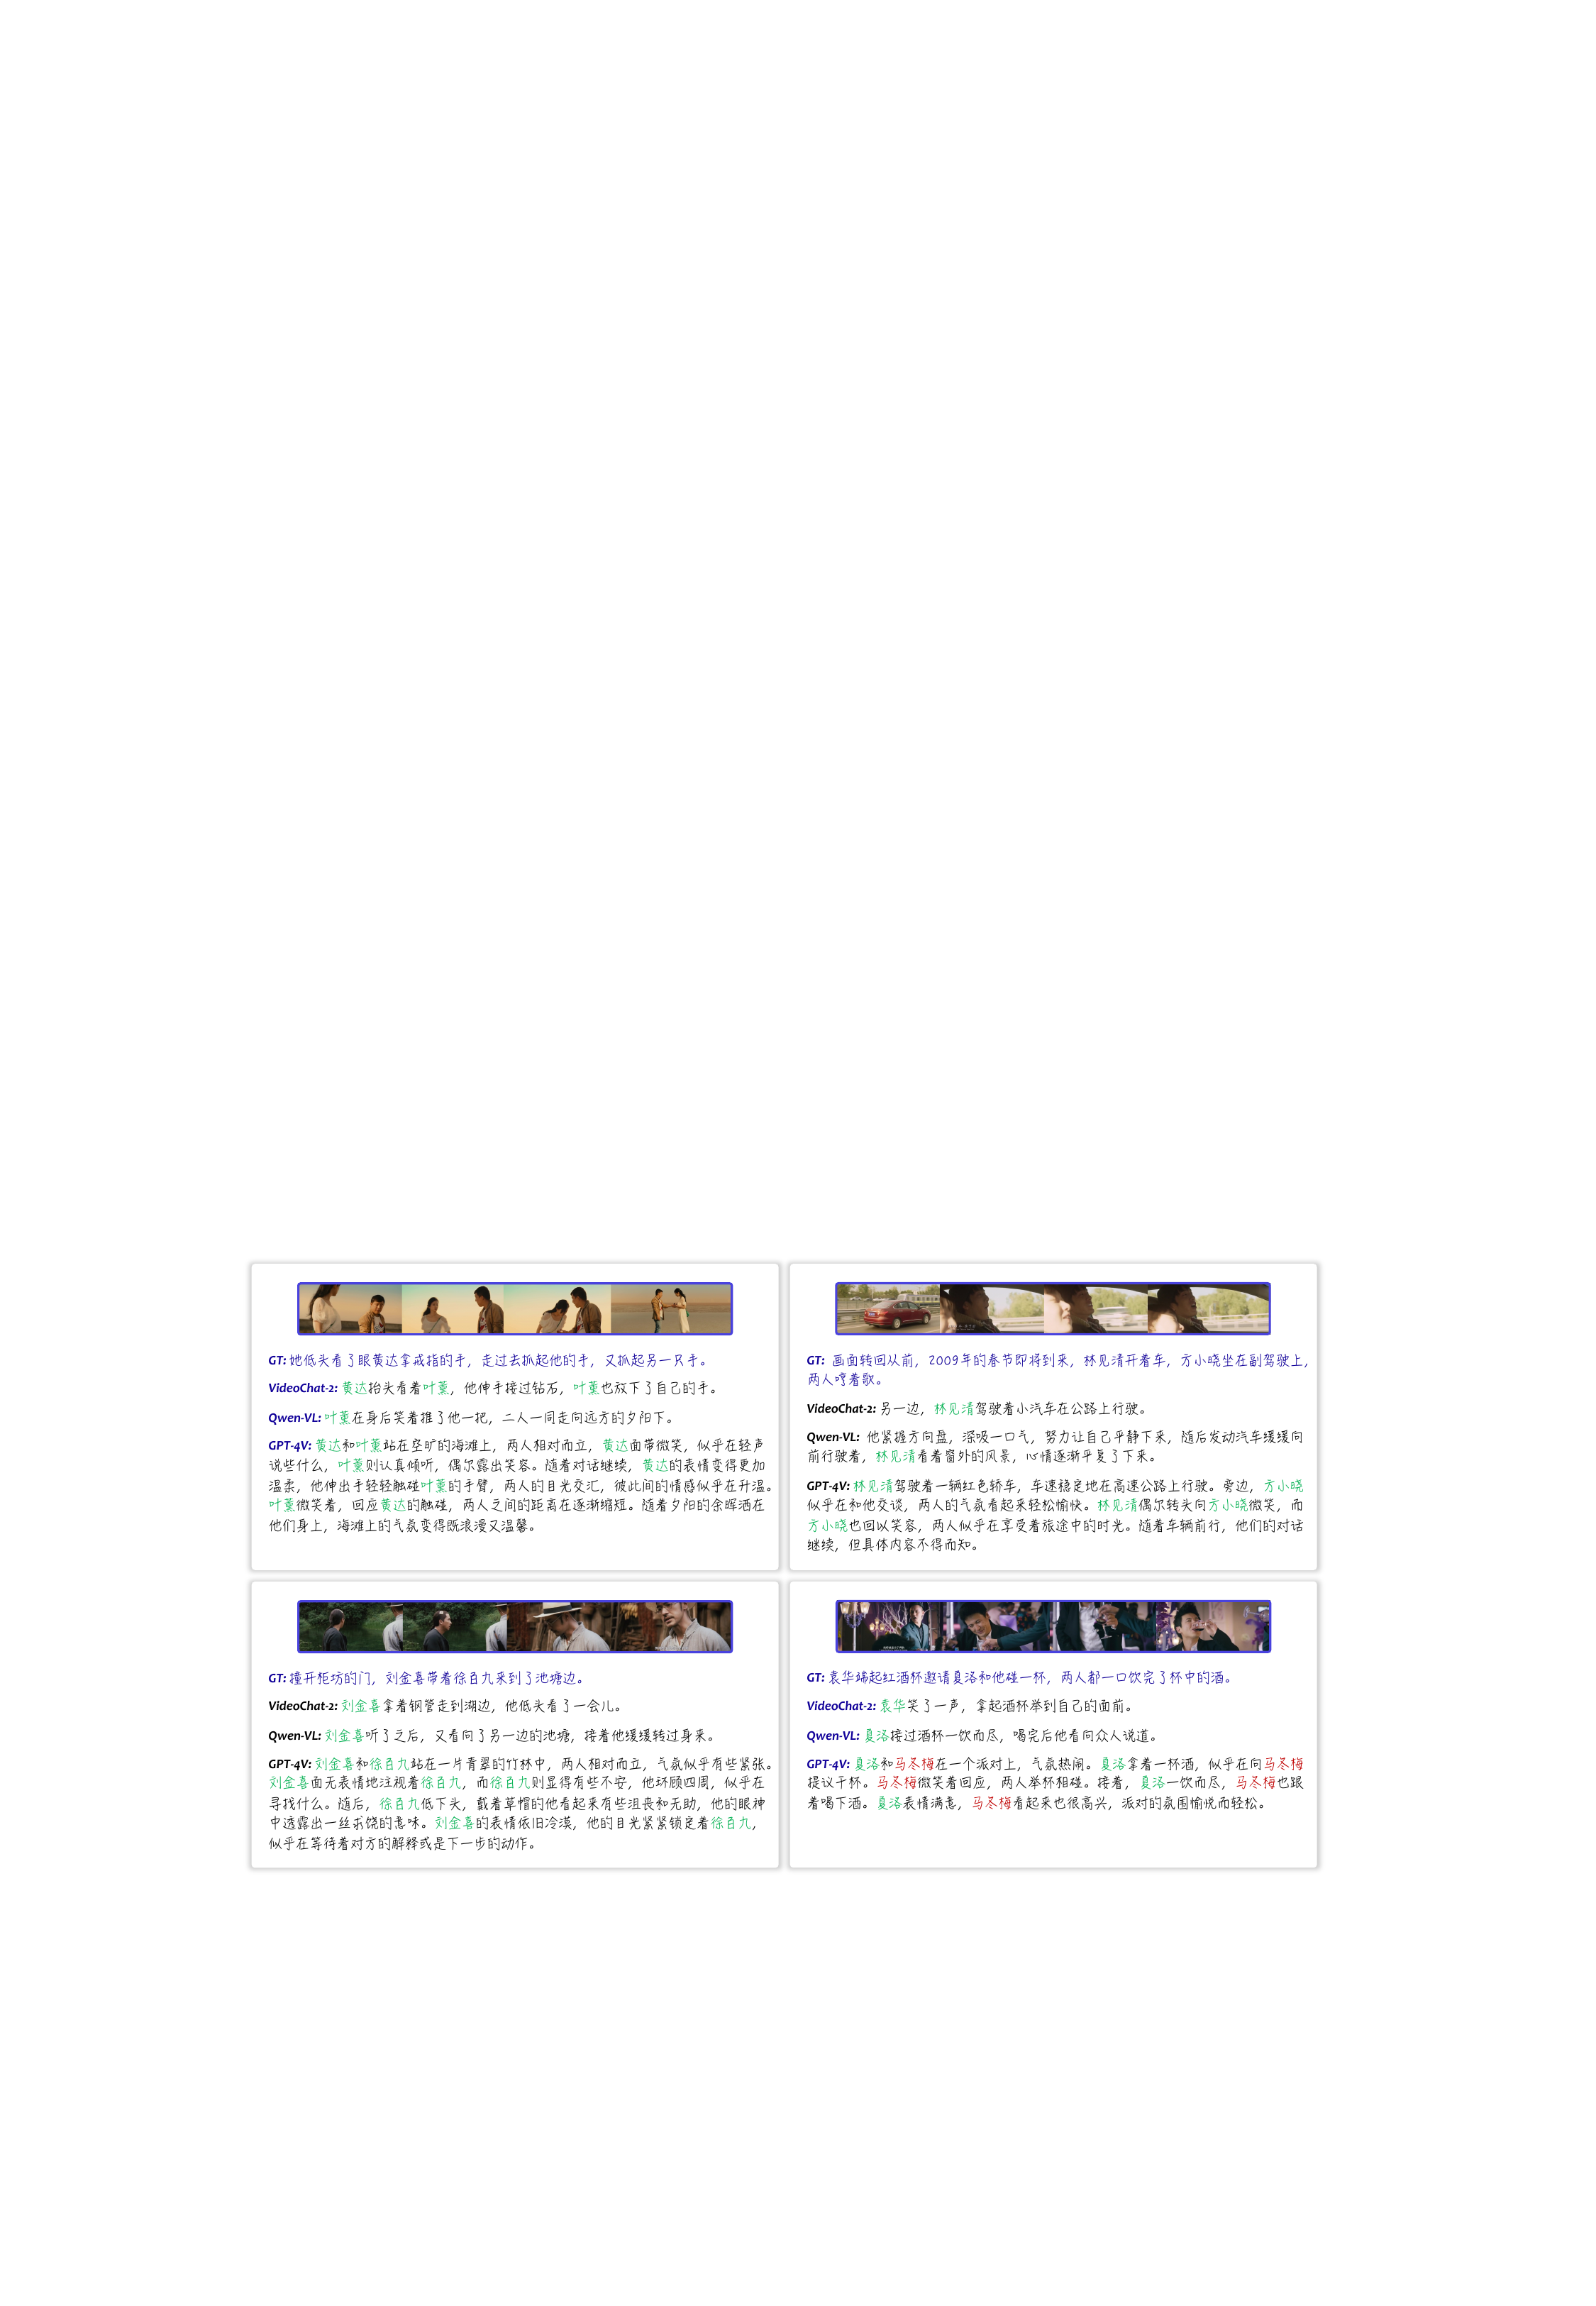}
    \end{center}
    % \vspace{-8pt}
\caption{Qualitative results from our baseline models on Movie101v2-zh.}
\label{fig:supp-qualitative-zh}
% \vspace{-8pt}
\end{figure*}
